# Supplementary material for: Improving Interpretability of Deep Sequential Knowledge Tracing Models with Question-centric Cognitive Representations
Source: arXiv:2302.06885 source file (2023-03-16)
Supplement: Supplementary file 1 [file appendix.tex]

\subsection{A1. Iterative update equations for question-agnostic knowledge state ($\mathbf{g}_t$).}

Similar to the iterative update of student's question-level knowledge state ($\mathbf{a}_t$), we choose to use the LSTM cell to update the question-agnostic knowledge state ($\mathbf{g}_t$) after answering each question at timestamp $t$:

\begin{align*}
\mathbf{i}_{t} & = \sigma\left(\mathbf{W}_5 \cdot \mathbf{c}_t +\mathbf{U}_5 \cdot \mathbf{g}_{t-1}+\mathbf{b}_5\right) \\
\mathbf{f}_{t} & = \sigma\left(\mathbf{W}_6 \cdot \mathbf{c}_t +\mathbf{U}_6 \cdot \mathbf{g}_{t-1}+\mathbf{b}_6\right) \\
\mathbf{o}_{t} & = \sigma\left(\mathbf{W}_7 \cdot \mathbf{c}_t +\mathbf{U}_7 \cdot \mathbf{g}_{t-1}+\mathbf{b}_7\right) \\
\mathbf{\tilde{c}}_{t} & = \sigma\left(\mathbf{W}_8 \cdot \mathbf{c}_t +\mathbf{U}_8 \cdot \mathbf{g}_{t-1}+\mathbf{b}_8\right) \\
\mathbf{c}_{t} & = \mathbf{f}_{t} \odot \mathbf{c}_{t-1}+\mathbf{i}_{t} \odot \mathbf{\tilde{c}}_{t} \\
\mathbf{g}_t & = \mathbf{o}_{t} \odot \tanh \left(\mathbf{c}_{t}\right) 
\end{align*}

\noindent where $\mathbf{W}_5$, $\mathbf{W}_6$, $\mathbf{W}_7$, $\mathbf{W}_8$, $\mathbf{U}_5$, $\mathbf{U}_6$, $\mathbf{U}_7$, $\mathbf{U}_8$, $\mathbf{b}_5$, $\mathbf{b}_6$, $\mathbf{b}_7$, $\mathbf{b}_8$ are trainable parameters and $\mathbf{W}_i \in \mathbb{R}^{d \times 2d}$, $\mathbf{U}_i \in \mathbb{R}^{d \times d}$, $\mathbf{b}_i \in \mathbb{R}^{d \times 1}$ and $i = 5, 6, 7, 8$.

\subsection{A2. Overall performance in terms of accuracy.}

The overall results (with standard deviation) of all baselines with our proposed QIKT model on three datasets are reported in Table \ref{tab:overall_acc}. We found in ASSIST2009 and Algebra2005 datasets that the best result is AKT, IEKT, respectively. That is because the dataset's distribution easily influences the accuracy metric. Such as student's correctness ratio is 0.6582, 0.7553 and 0.5373 on ASSIST2009, Algebra2005 and NeruIP34, respectively. We use a default threshold of 0.5 to decide whether the model's prediction is correct or wrong. We do not tune the threshold, and this will bring some perturbation in the final result. Thus, we believe in this scenario, the AUC is a better metric to evaluate models' performance.

% Please add the following required packages to your document preamble:
% \usepackage{multirow}
\begin{table*}[!hptb]\small
\centering
\caption{The overall prediction performance of all the baseline models and our QIKT in terms of \emph{accuracy}. We highlight the highest results with bold.}
\label{tab:overall_acc}
\begin{tabular}{c|c|c|c|c|ccc}
\toprule	
\multirow{2}{*}{Method} & \multirow{2}{*}{Model Type} & \multirow{2}{*}{\begin{tabular}[c]{@{}c@{}}Usage of \\ Questions\end{tabular}} & \multirow{2}{*}{\begin{tabular}[c]{@{}c@{}}Usage of \\ KCs\end{tabular}} & \multirow{2}{*}{\begin{tabular}[c]{@{}c@{}}Is \\ interpretable\end{tabular}} & \multicolumn{3}{c}{ACC}         \\  \cline{6-8}                                                
                        &                       &                                                                           &                                                                          &                                                                              & ASSIST2009             & Algebra2005            & NeurIPS34              \\
\hline
DKT                     & Sequential            & No                                                                        & Yes                                                                      & No                                                                           & 0.7243±0.0014                  & 0.8097±0.0005                   & 0.7032±0.0004                 \\
DKT+                    & Sequential            & No                                                                        & Yes                                                                      & No                                                                           & 0.7248±0.0009                  & 0.8097±0.0007                   & 0.7039±0.0004                 \\
KQN                     & Sequential            & No                                                                        & Yes                                                                      & No                                                                           & 0.7228±0.0009                  & 0.8025±0.0006                   & 0.7028±0.0001                 \\
qDKT                    & Sequential            & Yes                                                                       & No                                                                       & No                                                                           & 0.6787±0.0039                  & 0.7262±0.0012                   & 0.7299±0.0007                 \\
DKT-IRT                 & Sequential            & No                                                                        & Yes                                                                      & Yes                                                                          & 0.7266±0.0005                  & 0.8173±0.0005                   & 0.7041±0.0007                 \\
IEKT                    & Sequential            & Yes                                                                       & Yes                                                                      & No                                                                           & 0.7375±0.0042                  & \textbf{0.8236±0.0010}          & 0.7330±0.0002                 \\
DeepIRT                 & Memory                & No                                                                        & Yes                                                                      & Yes                                                                          & 0.7195±0.0004                  & 0.8037±0.0009                   & 0.7014±0.0008                 \\
DKVMN                   & Memory                & No                                                                        & Yes                                                                      & No                                                                           & 0.7198±0.0010                  & 0.8027±0.0006                   & 0.7016±0.0005                 \\
ATKT                    & Adversarial           & No                                                                        & Yes                                                                      & No                                                                           & 0.7208±0.0009                  & 0.7998±0.0019                   & 0.7013±0.0002                 \\
GKT                     & Graph                 & No                                                                        & Yes                                                                      & No                                                                           & 0.7153±0.0032                  & 0.8088±0.0008                   & 0.7014±0.0028                 \\
SAKT                    & Attention             & No                                                                        & Yes                                                                      & No                                                                           & 0.7063±0.0018                  & 0.7954±0.0020                   & 0.6879±0.0004                 \\
SAINT                   & Attention             & Yes                                                                       & Yes                                                                      & No                                                                           & 0.6935±0.0034                  & 0.7791±0.0016                   & 0.7180±0.0006                 \\
AKT                     & Attention             & Yes                                                                       & Yes                                                                      & No                                                                           & \textbf{0.7392±0.0021}         & 0.8124±0.0011                   & 0.7323±0.0005                 \\
\hline
QIKT                    & Sequential            & Yes                                                                       & Yes                                                                      & Yes                                                                          & 0.7381±0.0014                  & 0.8222±0.0006                   & \textbf{0.7333±0.0005}       \\
\bottomrule
\end{tabular}
\end{table*}

\subsection{A3. The detailed results of significant test on every model pair for all three datasets.}

We conduct the paired t-test on each pair of models on three datasets. The results in ASSIST2009, Algebra2005 and NeurIPS34 are listed on Tables \ref{tab:p_assist2009},\ref{tab:p_algebra2005} and \ref{tab:p_NeurIPS34}, respectively.

%assist2009

\begin{table*}[!hbpt]\tiny
\centering
\caption{The p-values between two pairs of models in the \emph{ASSIST2009} dataset. We highlight the p-values $\textgreater$ 0.01  with bold.}
\label{tab:p_assist2009}
\begin{tabular}{c|cccccccccccccc}
\toprule
{}        & DKT    & DKT+   & KQN    & qDKT   & DKT-IRT & IEKT   & DeepIRT         & DKVMN  & ATKT            & GKT    & SAKT   & SAINT  & AKT    & QIKT   \\
\hline
DKT     & -      & 0.0000 & 0.0000 & 0.0000 & 0.0000  & 0.0000 & 0.0000          & 0.0000 & 0.0000          & 0.0000 & 0.0000 & 0.0000 & 0.0000 & 0.0000 \\
DKT+    & 0.0000 & -      & 0.0000 & 0.0000 & 0.0000  & 0.0000 & 0.0000          & 0.0000 & 0.0000          & 0.0000 & 0.0000 & 0.0000 & 0.0000 & 0.0000 \\
KQN     & 0.0000 & 0.0000 & -      & 0.0000 & 0.0000  & 0.0000 & 0.0000          & 0.0000 & 0.0000          & 0.0000 & 0.0000 & 0.0000 & 0.0000 & 0.0000 \\
qDKT    & 0.0000 & 0.0000 & 0.0000 & -      & 0.0000  & 0.0000 & 0.0000          & 0.0000 & 0.0000          & 0.0000 & 0.0000 & 0.0000 & 0.0000 & 0.0000 \\
DKT-IRT & 0.0000 & 0.0000 & 0.0000 & 0.0000 & -       & 0.0012 & 0.0000          & 0.0000 & 0.0000          & 0.0000 & 0.0000 & 0.0000 & 0.0000 & 0.0000 \\
IEKT    & 0.0000 & 0.0000 & 0.0000 & 0.0000 & 0.0012  & -      & 0.0000          & 0.0000 & 0.0000          & 0.0000 & 0.0000 & 0.0000 & 0.0000 & 0.0000 \\
DeepIRT & 0.0000 & 0.0000 & 0.0000 & 0.0000 & 0.0000  & 0.0000 & -               & 0.0000 & \textbf{0.8252} & 0.0000 & 0.0000 & 0.0000 & 0.0000 & 0.0000 \\
DKVMN   & 0.0000 & 0.0000 & 0.0000 & 0.0000 & 0.0000  & 0.0000 & 0.0000          & -      & 0.0000          & 0.0000 & 0.0000 & 0.0000 & 0.0000 & 0.0000 \\
ATKT    & 0.0000 & 0.0000 & 0.0000 & 0.0000 & 0.0000  & 0.0000 & \textbf{0.8252} & 0.0000 & -               & 0.0000 & 0.0000 & 0.0000 & 0.0000 & 0.0000 \\
GKT     & 0.0000 & 0.0000 & 0.0000 & 0.0000 & 0.0000  & 0.0000 & 0.0000          & 0.0000 & 0.0000          & -      & 0.0000 & 0.0000 & 0.0000 & 0.0000 \\
SAKT    & 0.0000 & 0.0000 & 0.0000 & 0.0000 & 0.0000  & 0.0000 & 0.0000          & 0.0000 & 0.0000          & 0.0000 & -      & 0.0000 & 0.0000 & 0.0000 \\
SAINT   & 0.0000 & 0.0000 & 0.0000 & 0.0000 & 0.0000  & 0.0000 & 0.0000          & 0.0000 & 0.0000          & 0.0000 & 0.0000 & -      & 0.0000 & 0.0000 \\
AKT     & 0.0000 & 0.0000 & 0.0000 & 0.0000 & 0.0000  & 0.0000 & 0.0000          & 0.0000 & 0.0000          & 0.0000 & 0.0000 & 0.0000 & -      & 0.0000 \\
QIKT    & 0.0000 & 0.0000 & 0.0000 & 0.0000 & 0.0000  & 0.0000 & 0.0000          & 0.0000 & 0.0000          & 0.0000 & 0.0000 & 0.0000 & 0.0000 & -      \\
\bottomrule
\end{tabular}
\end{table*}

%Algebra2005

\begin{table*}[!hbpt]\tiny
\centering
\caption{The p-values between two pairs of models in the \emph{Algebra2005} dataset. We highlight the p-values $\textgreater$ 0.01  with bold.}
\label{tab:p_algebra2005}
\begin{tabular}{c|cccccccccccccc}
\toprule
{}        & DKT    & DKT+   & KQN    & qDKT   & DKT-IRT & IEKT   & DeepIRT & DKVMN           & ATKT   & GKT    & SAKT   & SAINT  & AKT             & QIKT   \\
\hline
DKT     & -      & 0.0000 & 0.0000 & 0.0000 & 0.0000  & 0.0000 & 0.0000  & 0.0000          & 0.0000 & 0.0000 & 0.0000 & 0.0000 & 0.0000          & 0.0000 \\
DKT+    & 0.0000 & -      & 0.0000 & 0.0000 & 0.0000  & 0.0000 & 0.0000  & 0.0000          & 0.0000 & 0.0000 & 0.0000 & 0.0000 & 0.0000          & 0.0000 \\
KQN     & 0.0000 & 0.0000 & -      & 0.0000 & 0.0000  & 0.0000 & 0.0000  & 0.0000          & 0.0000 & 0.0000 & 0.0000 & 0.0000 & 0.0000          & 0.0000 \\
qDKT    & 0.0000 & 0.0000 & 0.0000 & -      & 0.0000  & 0.0000 & 0.0000  & 0.0000          & 0.0000 & 0.0000 & 0.0000 & 0.0000 & 0.0000          & 0.0000 \\
DKT-IRT & 0.0000 & 0.0000 & 0.0000 & 0.0000 & -       & 0.0000 & 0.0000  & 0.0000          & 0.0000 & 0.0000 & 0.0000 & 0.0000 & 0.0000          & 0.0000 \\
IEKT    & 0.0000 & 0.0000 & 0.0000 & 0.0000 & 0.0000  & -      & 0.0000  & 0.0000          & 0.0000 & 0.0000 & 0.0000 & 0.0000 & 0.0000          & 0.0000 \\
DeepIRT & 0.0000 & 0.0000 & 0.0000 & 0.0000 & 0.0000  & 0.0000 & -       & 0.0000          & 0.0000 & 0.0000 & 0.0000 & 0.0000 & 0.0000          & 0.0000 \\
DKVMN   & 0.0000 & 0.0000 & 0.0000 & 0.0000 & 0.0000  & 0.0000 & 0.0000  & -               & 0.0000 & 0.0000 & 0.0000 & 0.0000 & \textbf{0.3070} & 0.0000 \\
ATKT    & 0.0000 & 0.0000 & 0.0000 & 0.0000 & 0.0000  & 0.0000 & 0.0000  & 0.0000          & -      & 0.0000 & 0.0000 & 0.0000 & 0.0000          & 0.0000 \\
GKT     & 0.0000 & 0.0000 & 0.0000 & 0.0000 & 0.0000  & 0.0000 & 0.0000  & 0.0000          & 0.0000 & -      & 0.0000 & 0.0000 & 0.0000          & 0.0000 \\
SAKT    & 0.0000 & 0.0000 & 0.0000 & 0.0000 & 0.0000  & 0.0000 & 0.0000  & 0.0000          & 0.0000 & 0.0000 & -      & 0.0000 & 0.0000          & 0.0000 \\
SAINT   & 0.0000 & 0.0000 & 0.0000 & 0.0000 & 0.0000  & 0.0000 & 0.0000  & 0.0000          & 0.0000 & 0.0000 & 0.0000 & -      & 0.0000          & 0.0000 \\
AKT     & 0.0000 & 0.0000 & 0.0000 & 0.0000 & 0.0000  & 0.0000 & 0.0000  & \textbf{0.3070} & 0.0000 & 0.0000 & 0.0000 & 0.0000 & -               & 0.0000 \\
QIKT    & 0.0000 & 0.0000 & 0.0000 & 0.0000 & 0.0000  & 0.0000 & 0.0000  & 0.0000          & 0.0000 & 0.0000 & 0.0000 & 0.0000 & 0.0000          & -      \\
\bottomrule
\end{tabular}
\end{table*}

%NeurIPS34

\begin{table*}[!hbpt]\tiny
\centering
\caption{The p-values between two pairs of models in the \emph{NeurIPS34} dataset. We highlight the p-values $\textgreater$ 0.01  with bold.}
\label{tab:p_NeurIPS34}
\begin{tabular}{c|cccccccccccccc}
\toprule
{}        & DKT    & DKT+            & KQN    & qDKT   & DKT-IRT & IEKT            & DeepIRT & DKVMN           & ATKT   & GKT             & SAKT   & SAINT  & AKT    & QIKT   \\ \hline

DKT     & -      & 0.0000          & 0.0000 & 0.0000 & 0.0000  & 0.0000          & 0.0000  & 0.0000          & 0.0000 & 0.0000          & 0.0000 & 0.0000 & 0.0000 & 0.0000 \\
DKT+    & 0.0000 & -               & 0.0000 & 0.0000 & 0.0000  & 0.0000          & 0.0000  & 0.0000          & 0.0000 & \textbf{0.5937} & 0.0000 & 0.0000 & 0.0000 & 0.0000 \\
KQN     & 0.0000 & 0.0000          & -      & 0.0000 & 0.0000  & 0.0000          & 0.0000  & 0.0000          & 0.0000 & 0.0000          & 0.0000 & 0.0000 & 0.0000 & 0.0000 \\
qDKT    & 0.0000 & 0.0000          & 0.0000 & -      & 0.0000  & 0.0000          & 0.0000  & 0.0000          & 0.0000 & 0.0000          & 0.0000 & 0.0000 & 0.0000 & 0.0000 \\
DKT-IRT & 0.0000 & 0.0000          & 0.0000 & 0.0000 & -       & 0.0000          & 0.0000  & 0.0000          & 0.0000 & 0.0000          & 0.0000 & 0.0000 & 0.0000 & 0.0000 \\
IEKT    & 0.0000 & 0.0000          & 0.0000 & 0.0000 & 0.0000  & -               & 0.0000  & \textbf{0.0871} & 0.0000 & 0.0000          & 0.0000 & 0.0000 & 0.0000 & 0.0000 \\
DeepIRT & 0.0000 & 0.0000          & 0.0000 & 0.0000 & 0.0000  & 0.0000          & -       & 0.0000          & 0.0000 & 0.0000          & 0.0000 & 0.0000 & 0.0000 & 0.0000 \\
DKVMN   & 0.0000 & 0.0000          & 0.0000 & 0.0000 & 0.0000  & \textbf{0.0871} & 0.0000  & -               & 0.0000 & 0.0000          & 0.0000 & 0.0000 & 0.0000 & 0.0000 \\
ATKT    & 0.0000 & 0.0000          & 0.0000 & 0.0000 & 0.0000  & 0.0000          & 0.0000  & 0.0000          & -      & 0.0000          & 0.0000 & 0.0000 & 0.0000 & 0.0000 \\
GKT     & 0.0000 & \textbf{0.5937} & 0.0000 & 0.0000 & 0.0000  & 0.0000          & 0.0000  & 0.0000          & 0.0000 & -               & 0.0000 & 0.0000 & 0.0000 & 0.0000 \\
SAKT    & 0.0000 & 0.0000          & 0.0000 & 0.0000 & 0.0000  & 0.0000          & 0.0000  & 0.0000          & 0.0000 & 0.0000          & -      & 0.0000 & 0.0000 & 0.0000 \\
SAINT   & 0.0000 & 0.0000          & 0.0000 & 0.0000 & 0.0000  & 0.0000          & 0.0000  & 0.0000          & 0.0000 & 0.0000          & 0.0000 & -      & 0.0000 & 0.0000 \\
AKT     & 0.0000 & 0.0000          & 0.0000 & 0.0000 & 0.0000  & 0.0000          & 0.0000  & 0.0000          & 0.0000 & 0.0000          & 0.0000 & 0.0000 & -      & 0.0000 \\
QIKT    & 0.0000 & 0.0000          & 0.0000 & 0.0000 & 0.0000  & 0.0000          & 0.0000  & 0.0000          & 0.0000 & 0.0000          & 0.0000 & 0.0000 & 0.0000 & -      \\
\bottomrule
\end{tabular}
\end{table*}

\subsection{A4. The visualization of QIKT and different modules' output.}
As discussed in Section \ref{sec:results}. Here we report the outputs of QIKT and KA, KS and PS modules for six students in Figure \ref{fig:all_y}.

\begin{figure}[!bpht]
     \centering
     \begin{subfigure}[b]{0.47\textwidth}
         \centering
         \includegraphics[width=\textwidth]{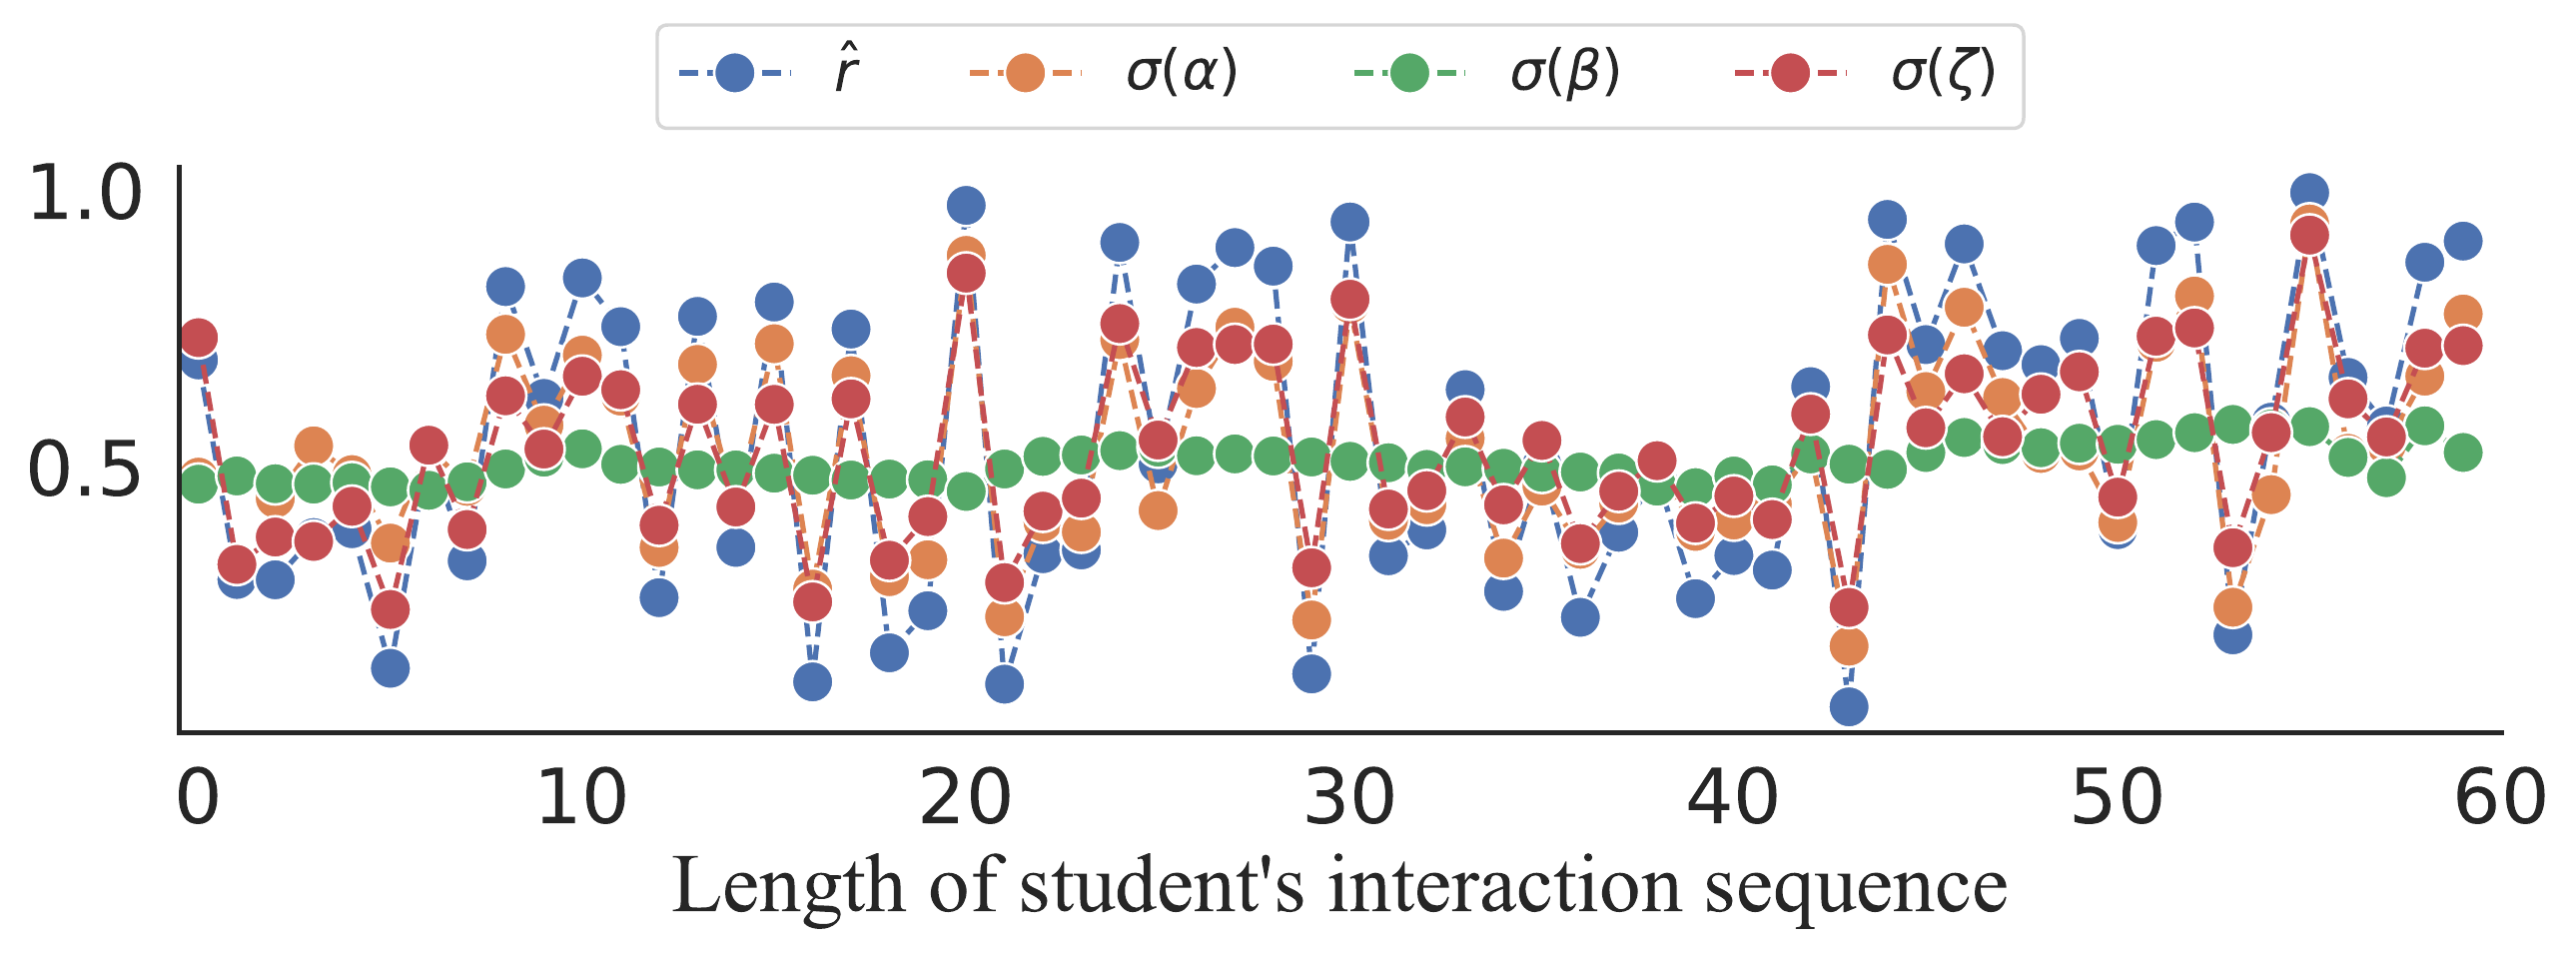}         \caption{Student 1}
         \label{fig:visual_y_a_1}
     \end{subfigure}
%     \hfill
     \begin{subfigure}[b]{0.47\textwidth}
         \centering
         \includegraphics[width=\textwidth]{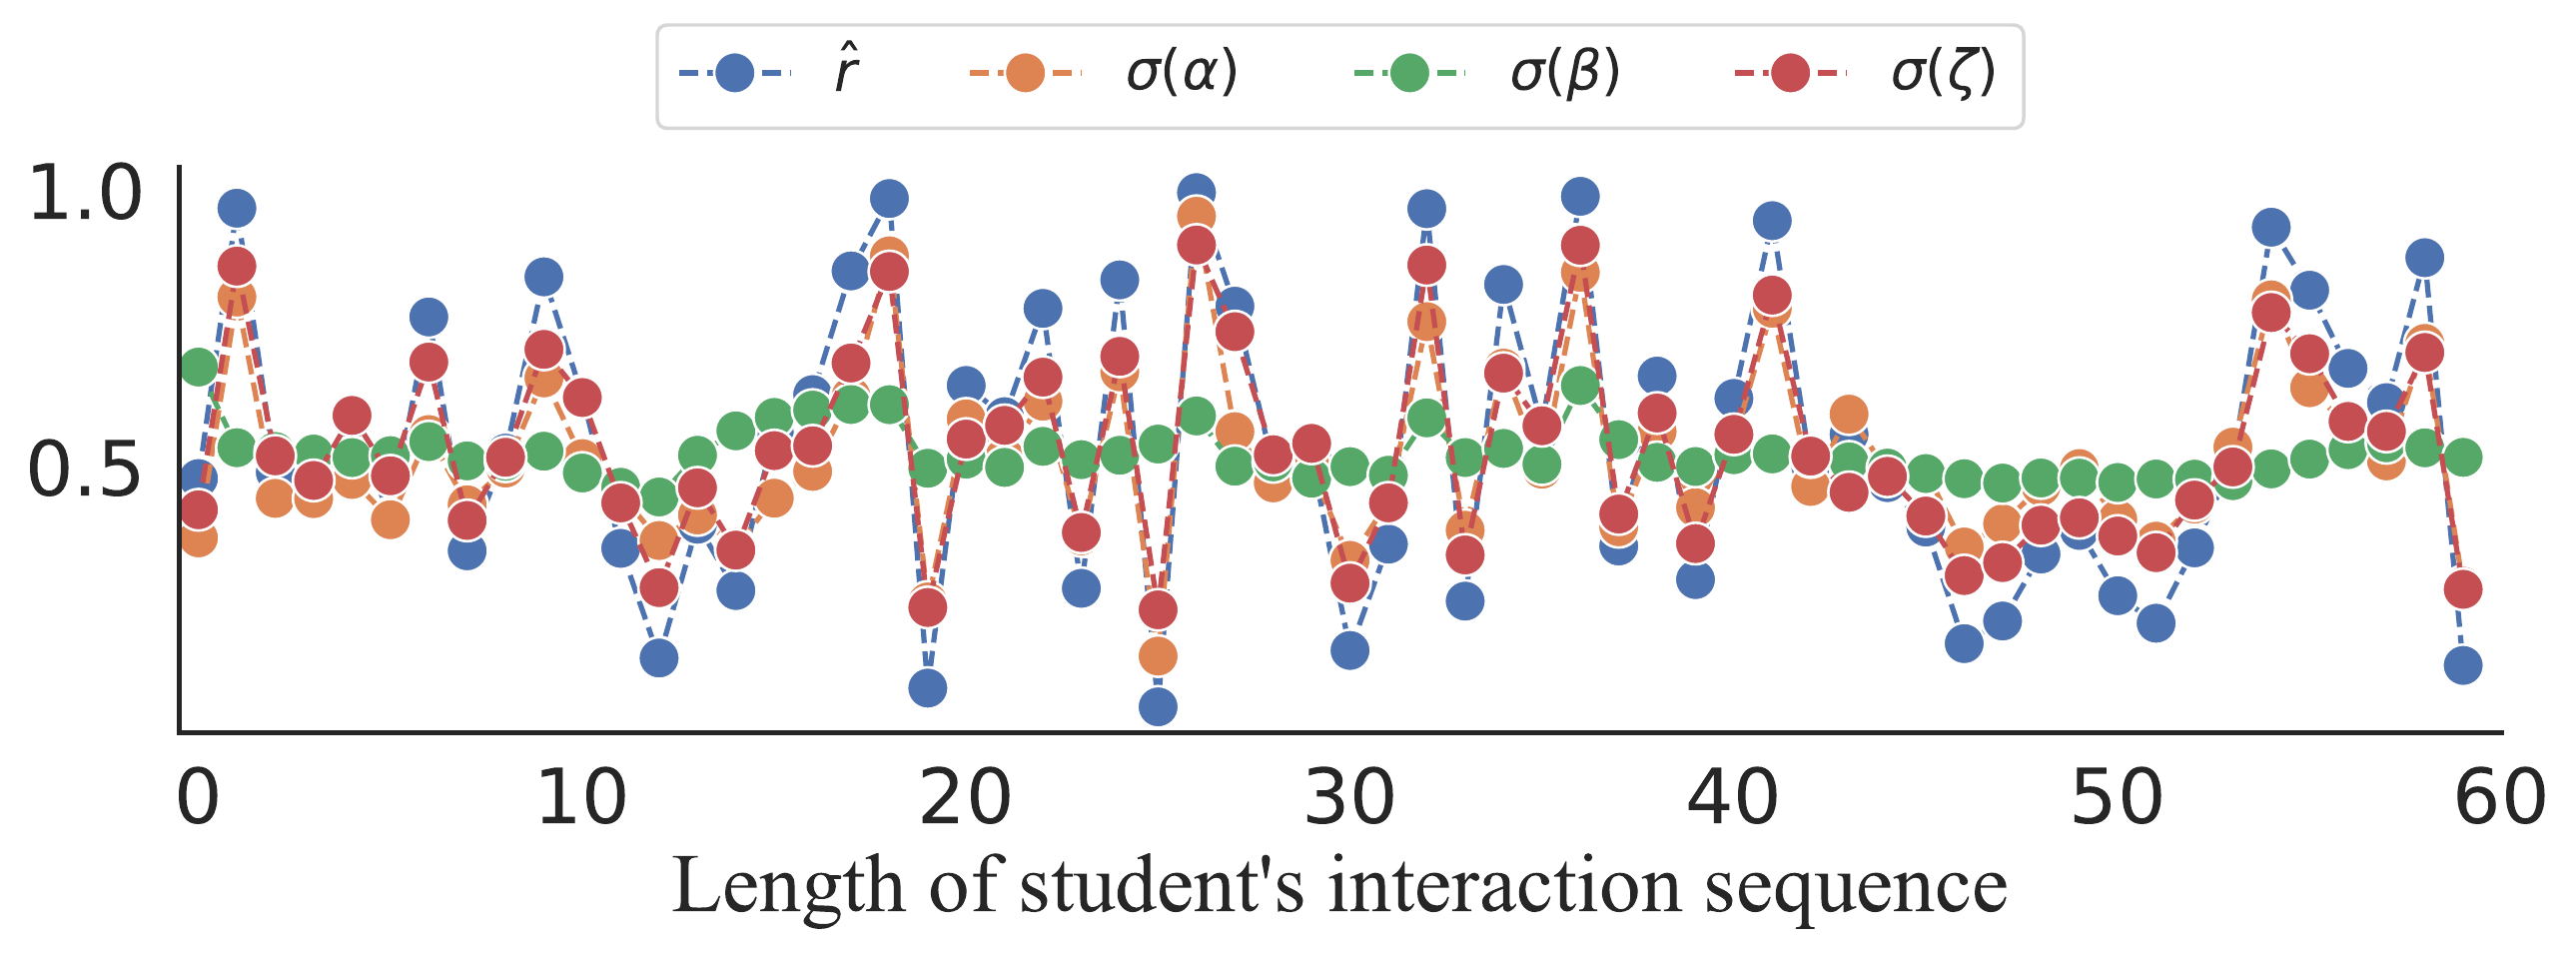}
         \caption{Student 2}
         \label{fig:visual_y_a_2}
     \end{subfigure}
     \begin{subfigure}[b]{0.47\textwidth}
         \centering
         \includegraphics[width=\textwidth]{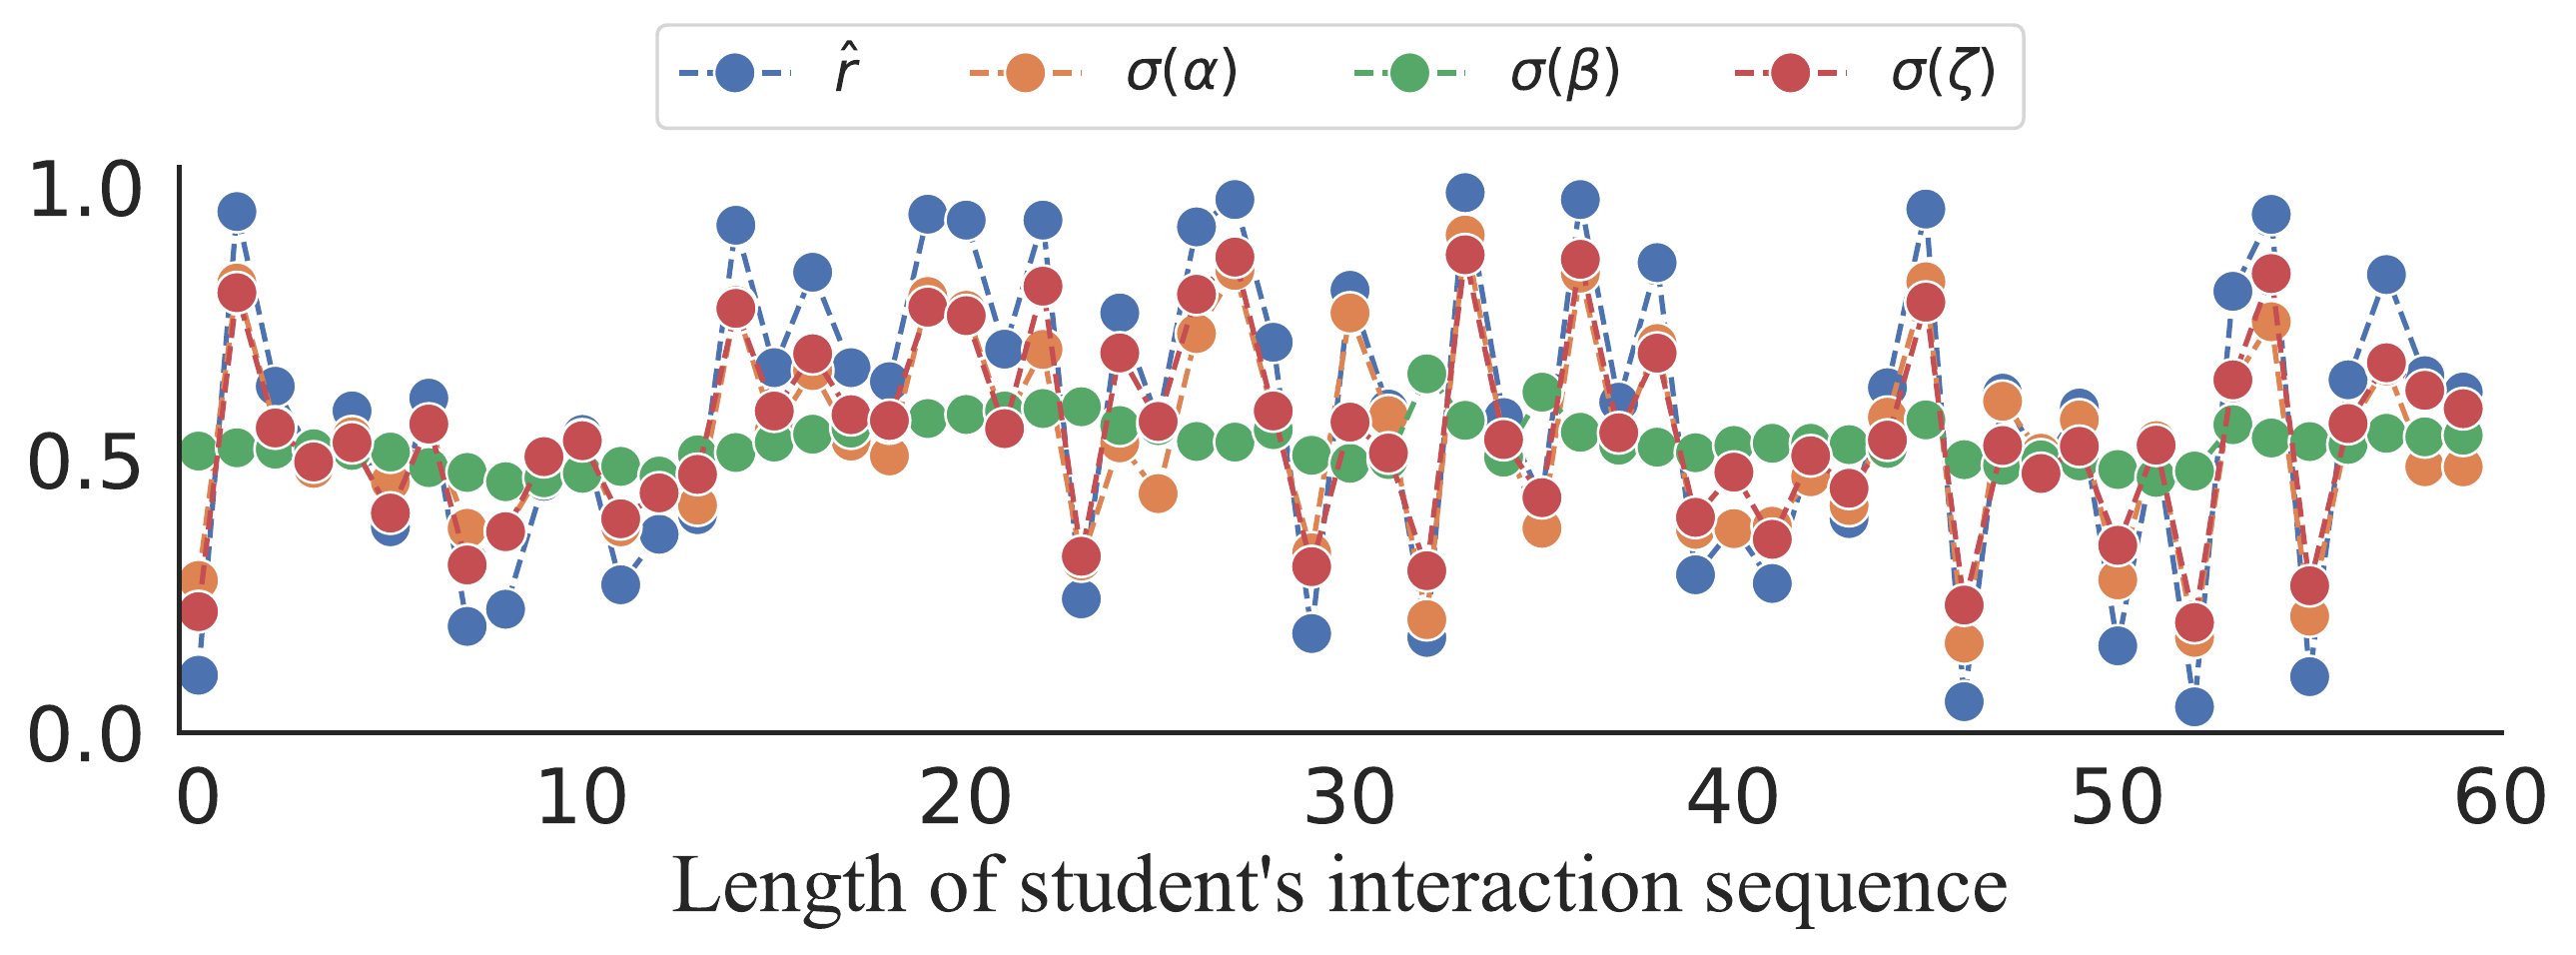}
         \caption{Student 3}
         \label{fig:visual_y_a_3}
     \end{subfigure}
     \begin{subfigure}[b]{0.47\textwidth}
         \centering
         \includegraphics[width=\textwidth]{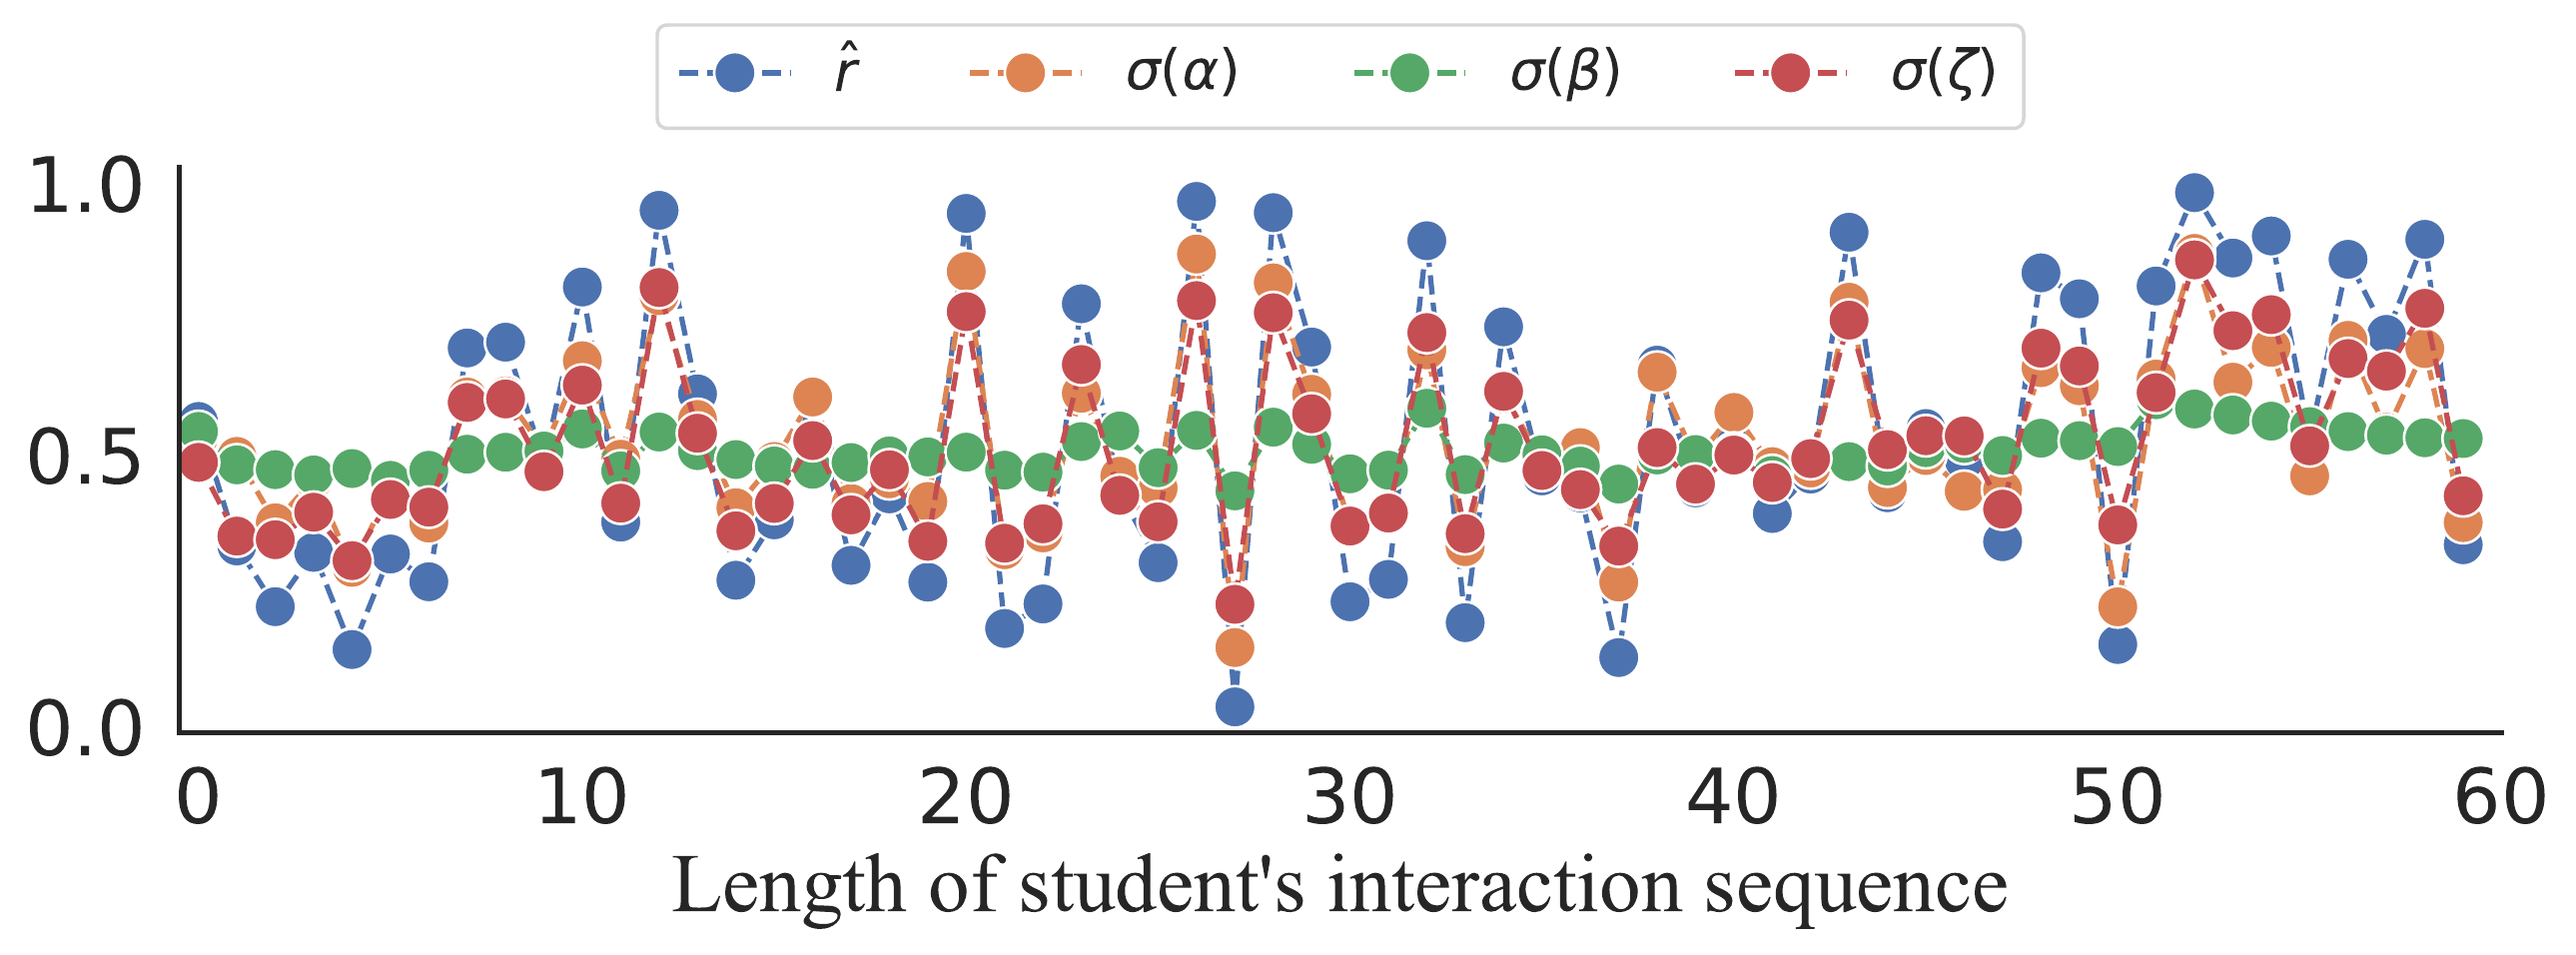}
         \caption{Student 4}
         \label{fig:visual_y_a_4}
     \end{subfigure}
     \begin{subfigure}[b]{0.47\textwidth}
         \centering
         \includegraphics[width=\textwidth]{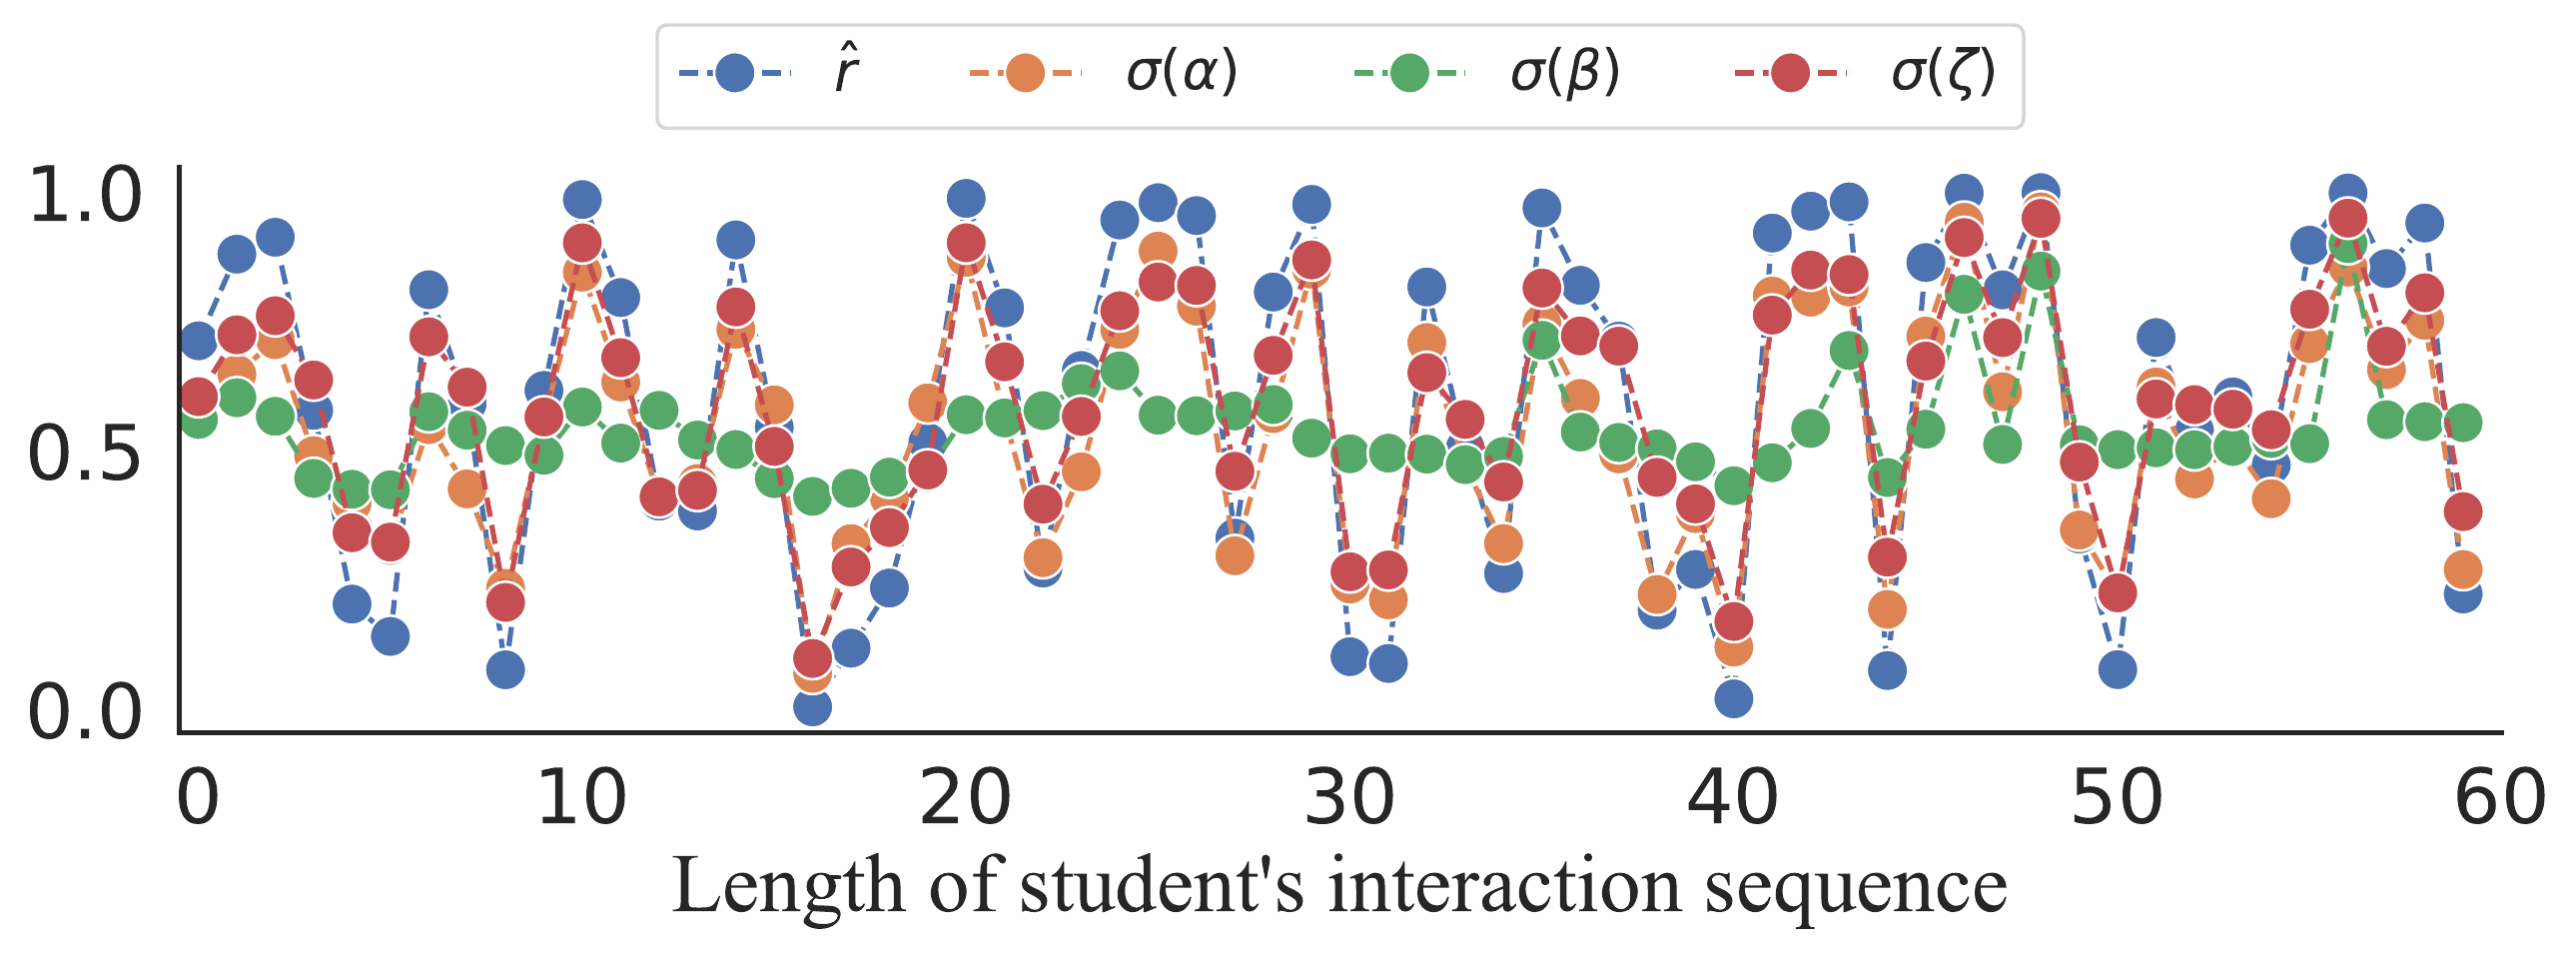}
         \caption{Student 5}
         \label{fig:visual_y_a_5}
     \end{subfigure}
     \begin{subfigure}[b]{0.47\textwidth}
         \centering
         \includegraphics[width=\textwidth]{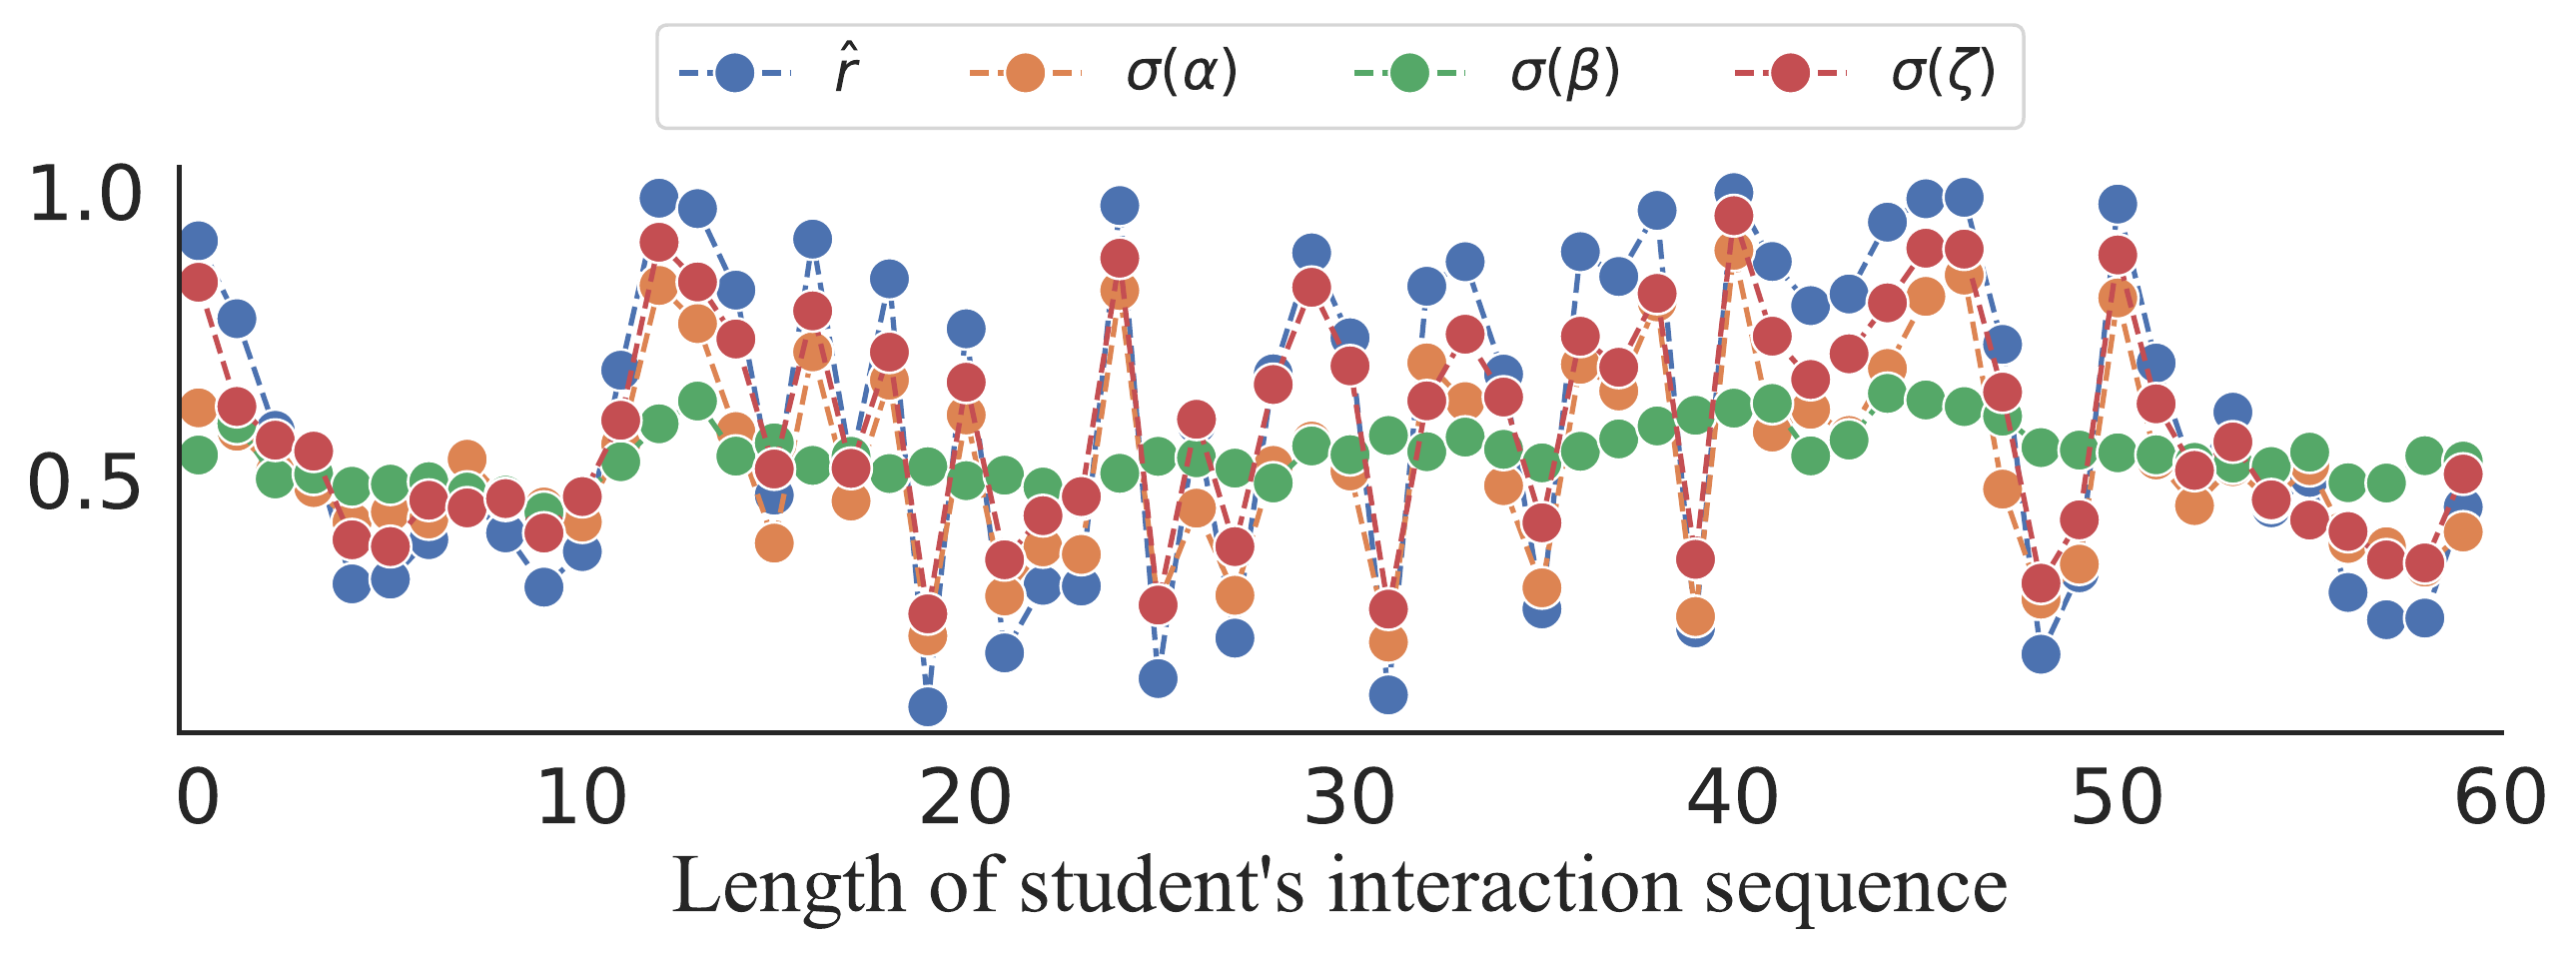}
         \caption{Student 6}
         \label{fig:visual_y_a_6}
     \end{subfigure}
%     \hfill
     \caption{The outputs of QIKT, KA module,KS module and PS module, i.e. $\hat{r}$, $\sigma{(\alpha)}$,$\sigma{(\beta)}$ and $\sigma{(\zeta)}$ at each steps in six students' interaction sequence.}
     \label{fig:all_y}
\end{figure}
